# Supplementary material for: High contrast qubit interactions using multimode cavity QED
Source: arXiv:1402.7036 ancillary file (2014-10-22)
Supplement: Supplementary file 1 [file multipole_supp.pdf]

# Supplementary Information for “High contrast qubit interactions using multimode cavity QED”

David C. McKay,<sup>1,\*</sup> Ravi Naik,<sup>1</sup> Philip Reinhold,<sup>1,†</sup> Lev S. Bishop,<sup>2,3</sup> and David I. Schuster<sup>1</sup>

<sup>1</sup>*James Franck Institute and Department of Physics, University of Chicago, Chicago, Illinois 60637*

<sup>2</sup>*Condensed Matter Theory Center, Department of Physics,  
University of Maryland, College Park, MD 20742, USA*

<sup>3</sup>*IBM T.J. Watson Research Center, Yorktown Heights, New York 10598, USA*

(Dated: October 2014)

## I. DERIVING THE DISPERSIVE HAMILTONIAN

The full Hamiltonian for the qubit-filter system (Eqns.1–4 in the main text) is

$$\hat{H} = \hat{H}_Q + \hat{H}_F + \hat{H}_{Q-F}, \quad (1)$$

$$\hat{H}_Q = h\nu_{Q,1} \frac{\hat{\sigma}_1^Z}{2} + h\nu_{Q,2} \frac{\hat{\sigma}_2^Z}{2}, \quad (2)$$

$$\hat{H}_F = \sum_{i=1}^n h\nu_F \hat{a}_i^\dagger \hat{a}_i + \sum_{i=2}^n hg_F (\hat{a}_i^\dagger \hat{a}_{i-1} + \hat{a}_{i-1}^\dagger \hat{a}_i), \quad (3)$$

$$\begin{aligned} \hat{H}_{Q-F} = & hg_{Q1,F} (\hat{a}_1^\dagger \hat{\sigma}_1^- + \hat{a}_1 \hat{\sigma}_1^+) + \\ & hg_{Q2,F} (\hat{a}_n^\dagger \hat{\sigma}_2^- + \hat{a}_n \hat{\sigma}_2^+). \end{aligned} \quad (4)$$

First, we can diagonalize the filter Hamiltonian (Eqn. 3), which is expressed in terms of the  $n$  bare resonator modes  $\hat{a}_i$ . For a given  $n$  we can label the filter eigenstates with a list  $j = \{-(n-1)/2, \dots, (n-1)/2\}$  such that the eigenvalues are

$$\nu_{F,j} = \nu_F + 2g_F \sin\left(\frac{j\pi}{n+1}\right). \quad (5)$$

For example, if  $n = 3$  (as in our experiment),  $\nu = \nu_F, \nu_F \pm \sqrt{2}g_F$ . To calculate the interaction of the qubits with these filter modes we need to know the weight of the eigenstate in the end resonators (modes  $\hat{a}_1, \hat{a}_n$ ), i.e., if we represent the new states as

$$|\nu_{F,j}\rangle = \sum_{i=1}^n \alpha_{j,i} \hat{a}_i^\dagger |0\rangle \quad (6)$$

where  $|0\rangle$  is the state with no photons in any resonator, then we need to know  $\alpha_{j,1}$  and  $\alpha_{j,n}$ . These have analytic expressions,

$$|\alpha_{j,1}| = |\alpha_{j,n}| = \frac{\cos\left(\frac{j\pi}{n+1}\right)}{\sqrt{(n+1)/2}}, \quad (7)$$

$$\frac{\alpha_{j,1}\alpha_{j,n}}{|\alpha_{j,1}||\alpha_{j,n}|} = (-1)^j. \quad (8)$$

The full Hamiltonian in the filter basis is given as (let the filter mode operators be  $\hat{b}_j$ ),

$$\hat{H} = h\nu_{Q,1} \frac{\hat{\sigma}_1^Z}{2} + h\nu_{Q,2} \frac{\hat{\sigma}_2^Z}{2} + \sum_{j=1}^n h \left[ \nu_{F,j} \hat{b}_j^\dagger \hat{b}_j + g_{Q1,F} \alpha_{j,1} (\hat{b}_j^\dagger \hat{\sigma}_1^- + \hat{b}_j \hat{\sigma}_1^+) + g_{Q2,F} \alpha_{j,n} (\hat{b}_j^\dagger \hat{\sigma}_2^- + \hat{b}_j \hat{\sigma}_2^+) \right]. \quad (9)$$

---

\*Email: dcmckay@uchicago.edu

†Current address: Yale Department of Applied Physics, New Haven, CT 06511

In the filter basis, the qubits are directly coupled through each of the modes. If  $n = 1$  Eqn. 9 reduces to the standard cavity QED Hamiltonian for two qubits coupled to a single cavity.

Next, we want to calculate the effective Hamiltonian for the qubit states ( $|gg\rangle, |eg\rangle, |ge\rangle, |ee\rangle$ ) in the dispersive limit ( $g_Q/\Delta, g_F/\Delta \ll 1$ ). The zeroth order qubit Hamiltonian is,

$$\hat{H}_{Q,0} = h\nu_{Q,1} \frac{\hat{\sigma}_1^Z}{2} + h\nu_{Q,2} \frac{\hat{\sigma}_2^Z}{2} \quad (10)$$

and we add in the second part of the full Hamiltonian Eqn. 9 perturbatively. There are no first order perturbative terms, but to second order the state  $|eg\rangle$  (and similarly  $|ge\rangle$ ) become dressed by the filter

$$|eg\rangle_{(2)} = |eg\rangle_{(0)} + \sum_j \frac{g_{Q1,F}\alpha_{j,1}}{\nu_{Q1} - \nu_{F,j}} |gg\rangle \otimes \hat{b}_j^\dagger |0\rangle. \quad (11)$$

The state  $|ee\rangle$  also gets dressed,

$$|ee\rangle_{(2)} = |ee\rangle_{(0)} + \sum_j \frac{g_{Q1,F}\alpha_{j,1}}{\nu_{Q1} - \nu_{F,j}} |ge\rangle \otimes \hat{b}_j^\dagger |0\rangle + \frac{g_{Q2,F}\alpha_{j,n}}{\nu_{Q2} - \nu_{F,j}} |ge\rangle \otimes \hat{b}_j^\dagger |0\rangle. \quad (12)$$

We can now recalculate the second order Hamiltonian by applying these states (after proper orthogonalization) to Eqn. 9 and we get that,

$$\hat{H}_{Q,2} = (h\nu_{Q,1} + \delta\nu_{Q,1}) \frac{\hat{\sigma}_1^Z}{2} + (h\nu_{Q,2} + \delta\nu_{Q,2}) \frac{\hat{\sigma}_2^Z}{2} + hJ(\sigma_1^+ \sigma_2^- + \sigma_2^+ \sigma_1^-) \quad (13)$$

where the  $\delta$  terms are single qubit energy shifts (Stark shifts) and the exchange term is

$$J = \frac{1}{2} \sum_j (g_{Q1,F} g_{Q2,F} \alpha_{j,1} \alpha_{j,n}) \left( \frac{1}{\nu_{Q1} - \nu_{F,j}} + \frac{1}{\nu_{Q2} - \nu_{F,j}} \right) \quad (14)$$

For simplicity assume that  $g_{Q1,F} = g_{Q2,F} = g_Q$ ,  $\nu_{Q1} = \nu_{Q2} = \nu_Q$ ,  $\nu_Q - \nu_F = \Delta$ ,

$$J = g_Q^2 \sum_j \frac{\alpha_{j,1} \alpha_{j,n}}{\Delta - (\nu_{F,j} - \nu_F)} \quad (15)$$

Substituting in the filter formulas, Eqns. 5,7,8 we get,

$$J = \frac{2g_Q^2}{n+1} \sum_j \frac{(-1)^j \cos^2\left(\frac{j\pi}{n+1}\right)}{\Delta - 2g_F \sin\left(\frac{j\pi}{n+1}\right)} \quad (16)$$

$$\approx \frac{2g_Q^2}{\Delta(n+1)} \sum_{k=0} \sum_j \left[ (-1)^j \cos^2\left(\frac{j\pi}{n+1}\right) \right] \left[ \frac{2g_F}{\Delta} \sin\left(\frac{j\pi}{n+1}\right) \right]^k \quad (17)$$

if  $g_F/\Delta \ll 1$ . Because of the alternating sign, the first non-zero term of the  $k$  sum occurs when  $k = n - 1$ ,

$$J = \frac{g_Q^2}{g_F} \left( \frac{g_F}{\Delta} \right)^n \quad (18)$$

which reproduces Eqn. 6 from the main text.

If we go to fourth-order in perturbation theory we can also recover a C-Phase interaction term  $\xi = E_{|ee\rangle} + E_{|gg\rangle} - (E_{|ge\rangle} + E_{|eg\rangle})$ . This type of interaction is not possible from Eqn. 13 since the exchange term shifts the energies of  $|ge\rangle$  and  $|eg\rangle$ , after diagonalization, equally in opposite directions. Deriving an exact analytic expression for  $\xi$  is difficult because of the large number of terms in the fourth-order expansion. For a single cavity a good approximation is that,

$$\xi = \frac{4J^2}{\Delta} \quad (19)$$

where we use  $\bar{\nu}_Q = (\nu_{Q1} + \nu_{Q2})/2$  to calculate  $J$  and  $\Delta$ . A similar approximation works for the multipole filter, except for a factor  $n$ ,

$$\xi = \frac{4nJ^2}{\Delta} \quad (20)$$

which is given as Eqn. 7 in the main text. In Fig. 1, we compare the dispersive approximation for  $J$  and  $\xi$  to a numerical diagonalization of the full Hamiltonian Eqn. 1.

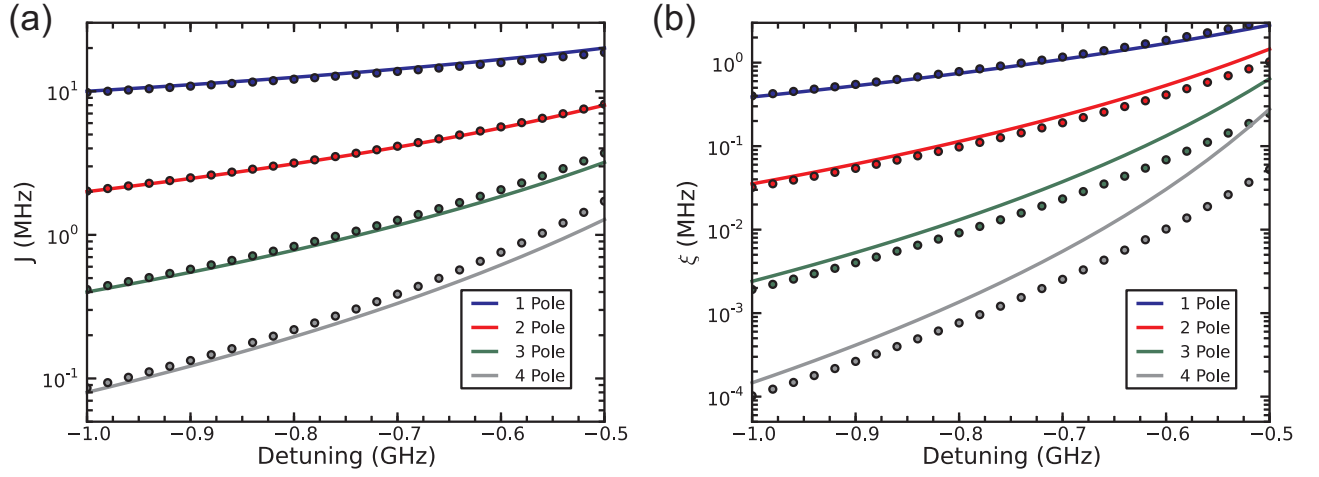

FIG. 1: Comparing our dispersive expressions for (a)  $J$  and (b)  $\xi$ , Eqns. 6,7 in the main text, to a numerical calculation from the full Hamiltonian Eqn. 1 using the parameters  $g_{Q1,F} = g_{Q2,F} = 100\text{MHz}$ ,  $g_F = 200\text{MHz}$  and  $\nu_F = 7\text{GHz}$ . (a)  $J$  calculated for different number of filter resonators  $n = 1 - 4$ . To calculate  $J$  numerically we take half the minimum spacing between the states  $|eg\rangle$  and  $|ge\rangle$ . The perturbative expression and the exact numerical value converge in the dispersive limit. (b)  $\xi$  calculated for  $n = 1 - 4$  with a detuning of  $200\text{MHz}$  between the qubits. The detuning from the filter  $\Delta$  is calculated with respect to the average qubit frequency. To calculate  $\xi$  we diagonalize the Hamiltonian and take  $\xi = E_{|ee\rangle'} + E_{|gg\rangle'} - E_{|ge\rangle'} - E_{|eg\rangle'}$  where  $|ee\rangle'$  is the state which adiabatically connects to  $|ee\rangle$  (and similarly for the other states). The agreement between the Eqn. 20 (Eqn. 7 in the main text) and the numerical calculation is not exact in the dispersive limit, but both display similar scaling with  $\Delta$ . In particular, the numerical calculation displays the same exponential suppression of  $\xi$  in the dispersive limit as is predicted by the approximate expression Eqn. 20.

## II. C-PHASE RATE QUBIT VS. TRANSMON

In the main text, we treat our device as a perfect two-level system, however, our device is a transmon qubit with a closely spaced third level ( $|f\rangle$ ). In the dispersive limit and when considering single excitations of the system, the qubit approach is adequate because the third level is far off-resonance. However, when both qubits are excited to the state  $|ee\rangle$  and brought into resonance with the filter, we must take the third level into consideration because the states  $|ee\rangle$ ,  $|gf\rangle$ ,  $|fg\rangle$  may have an avoided crossing. This scenario is true for our gate, and so, to calculate the C-Phase rate  $\xi$  numerically we must consider all three transmon levels. In Fig. 2, we calculate the C-Phase rate  $\xi$  as we ramp our two transmon qubits towards the filter (with one qubit lagging in frequency as in our experiment). We calculate  $\xi$  first treating it as a perfect qubit, and second including the third transmon level. We see that if our device were a true qubit, the C-Phase rate would continue to increase as we ramp both qubits through the filter and saturate at a value equal to the filter mode splitting (for  $n = 3$  this is  $\sqrt{2}g_F$ ). However, in the case of the transmon, the C-Phase rate peaks when the second qubit is just below the filter and then decreases when that qubit moves through the filter resonance. Although this is not a general feature of the C-Phase for the transmon - the exact C-Phase depends on how the two qubits are ramped with respect to each other - it demonstrates the importance of taking into account the higher transmon levels to understand the gate. Also, this type of C-Phase curve is a good description of the C-Phase expected for the ramp we use in our experiment, and is the motivation for leaving qubit 2 just below the filter resonance in our gate implementation.

## III. SAMPLE FABRICATION, DEVICE PARAMETERS, AND SETUP

Our multi-pole circuit QED device (Fig. 1 of the main text) was fabricated on  $450\mu\text{m}$  thick C-plane sapphire in a two-step process. In the first step, we deposited  $100\text{nm}$  of Nb using e-beam evaporation ( $0.9\text{nm/s}$ ) and performed optical lithography and reactive ion etch (RIE) to define all features of the circuit except the transmon. In the second step of our process, we used e-beam lithography (MMA-PMMA resist) and aluminum e-beam evaporation to construct the transmon (shunt capacitor plus junction). In order to form the junction, aluminum was first evaporated at  $0^\circ$  to a height of  $35\text{nm}$ , then the sample was oxidized in a  $\text{O}_2\text{-Ar}$  mixture (15/85) for 12 minutes at  $20\text{mBar}$ , and finally aluminum was evaporated at  $37^\circ$  to a height of  $120\text{nm}$  (Dolan bridge technique). The sample is mounted to a copper on arlon microwave board using GE varnish and electrically connected using Al wire bonds.

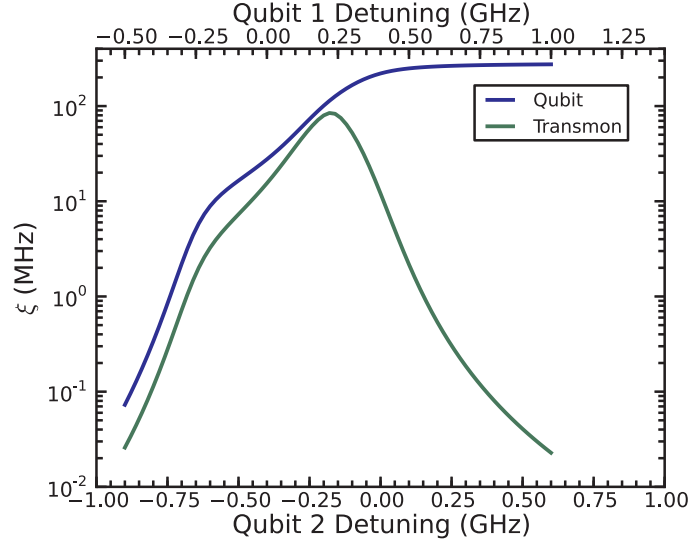

FIG. 2: C-Phase rate calculated for perfect qubits versus transmon qubits (i.e., including the next highest energy level) assuming perfect adiabaticity and for parameters  $g_{Q1,F} = g_{Q2,F} = 100\text{MHz}$ ,  $g_F = 200\text{MHz}$ ,  $\nu_F = 7\text{GHz}$ ,  $E_C = 200\text{MHz}$ .  $E_C$  sets the anharmonicity for the transmon device, such that  $E_{|f\rangle} - E_{|e\rangle} = E_{|e\rangle} - E_{|g\rangle} - E_C$ . In both calculations, the bare qubit 1 and qubit 2 frequencies are raised linearly with qubit 2 starting  $400\text{MHz}$  lower than qubit 1. To calculate  $\xi$  we diagonalize the Hamiltonian and take  $\xi = E_{|ee\rangle'} + E_{|gg\rangle'} - E_{|ge\rangle'} - E_{|eg\rangle'}$  where  $|ee\rangle'$  is the state which adiabatically connects to  $|ee\rangle$  (and similarly for the other states).

Detailed images of the lumped resonators and transmon are shown in Fig. 3. The resonators ( $(2\pi\nu)^2 = 1/LC$ ) are patterned during the optical lithography step and consist of two lumped shunt capacitors (of capacitance  $2C$ ) and a series inductor (of inductance  $L$ ) in a  $\pi$  configuration. The filter resonators have a resonance of  $\nu = 7.169\text{GHz}$  and a design impedance of  $100\text{ Ohms}$  and the readout resonators have frequencies of  $\nu = 4.20(4.65)\text{GHz}$  and design impedances of  $80\text{ Ohms}$ . Each transmon consists of two  $\approx 225\text{nm} \times 300\text{nm}$  Josephson junctions (i.e. total junction area is  $0.135\mu\text{m}^2$ ) in a DC SQUID loop. From two-tone spectroscopy of the transmon energy levels for qubit 1 (qubit 2) we measure  $E_J/h = 51.49(51.02)\text{GHz}$  (corresponding to  $I_C = 103.7(102.7)\text{nA}$ ), and  $E_C/h = 218.6(202.8)\text{MHz}$ . Each SQUID loop is located adjacent to a high speed flux line which can be utilized to tune the qubit frequency from the zero-flux transmon limit  $\nu = 9.36(8.89)\text{GHz}$  to the Cooper-pair limit  $4E_C$ . The flux line has tunability  $2.8(3.0)mA/\Phi_0$ . Each transmon is coupled to an individual readout resonator  $\nu_{read} = 4.1955(4.6564)\text{GHz}$  with  $Q = 13400(12100)$  and coupling rate  $g/h = 60(70)\text{MHz}$ .

Our cryogenic and measurement setup is illustrated in Fig. 4. Our sample is mounted inside an aluminum box which is enclosed in a light-tight cryoperm shield and heat sunk to the base stage of a dilution refrigerator (nominal temperature  $10\text{mK}$ ). Superconducting coaxial cable (NbTi) carries signals from the sample to a HEMT amplifier at  $4\text{K}$ . We primarily measure the transmission of the qubit readout resonator in homodyne configuration using a 1GSa/s ADC PCi card (Alazar ATS9870) connected to a standard desktop computer. The frequency and power of the readout tone is set to optimize the single shot fidelity discussion in § VIII.

#### IV. SINGLE QUBIT PROPERTIES

To probe the single qubit coherence properties we perform standard lifetime ( $T_1$ ) and Ramsey ( $T_2$ ) measurements of the individual qubits at the DC bias point for the experiments discussed in the main text  $\nu_{Q1,0}(\nu_{Q2,0}) = 6.2(6.4)\text{GHz}$ . Representative measurements for qubit 1 are shown in Fig. 5. We measure a  $e^{-1}$  lifetime for qubit 1 (qubit 2) of  $T_1 = 2.36(2.14)\mu\text{s}$ . We fit the Ramsey data to a Gaussian decay  $(e^{-t^2/2\sigma^2})[1]$  and measure  $\sigma = 312(492)\text{ns}$ .  $T_2^*$  can be expressed as  $T_2^* = 2\sigma$  (i.e., the slope when  $t = \sigma$ ). Assuming  $1/f$  flux noise, we estimate the flux noise density  $A$  from  $T_2^*$  and  $d\omega/d\Phi$  as  $A = 1.3(0.96) \times 10^{-5}\Phi_0$ , which is typical of these devices[2]. We note a small improvement in  $T_2^*$  if the fast-flux lines are terminated. The  $1/e$  decay time with spin echo and the flux lines terminated is  $1.6(1.3)\mu\text{s}$ .

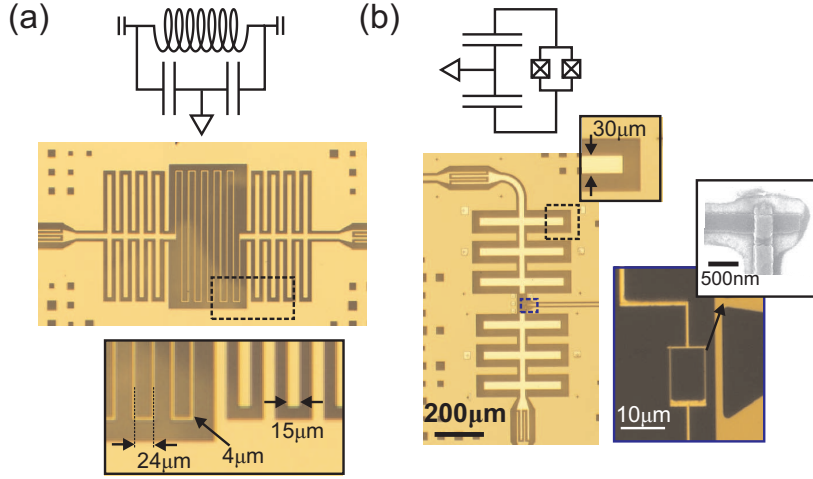

FIG. 3: (a) Schematic and optical image of the niobium-on-sapphire lumped resonators. The light color regions are niobium and the dark regions are sapphire. (b) Schematic and images of the transmon (from a comparable device). The junction image is taken with a scanning electron microscope; all other images are optical.

## V. FAST FLUX TUNING

To implement the gate discussed in the main text we require the ability to apply fast-flux pulses to the qubits while maintaining high DC flux bias stability when performing single qubit gates and to enable data averaging over hundreds of seconds. This second requirement is more demanding given that our DC flux bias point is on a large energy-flux slope (see Fig. 1 of the main text). In order to provide a highly stable DC flux bias and fast RF flux pulses with the lowest possible noise, we combine our DC flux bias and fast flux pulsing on a bias tee (Minicircuits ZX85-12G+). In addition we DC block the ground connection of the fast flux signal line to maintain an unambiguous return path for the DC flux bias.

The effect of these filtering components is a stable DC flux bias, however, there is significant pulse shaping of the fast-flux pulse. This shaping consists of both low pass filtering for signals  $>1\text{GHz}$ , and, more importantly, high pass filtering from the bias tee (200kHz cutoff). The high pass filtering results in a flux (qubit frequency) offset after the expected end of the flux pulse which persists for several microseconds. To compensate we apply additional flux pulsing after the main “gate” flux pulse. To calibrate these compensation pulses we perform time-resolved qubit spectroscopy[3].

## VI. FILTER LIFETIME

We measure the lifetime of the lowest filter mode by loading a single photon into the filter, waiting time  $\tau$  and retrieving the photon. To load the photon, we first excite qubit 1, then adiabatically ramp the qubit through the filter which creates a single photon in the lowest mode. We then bring qubit 1 back through the filter quickly, which leaves the photon in the filter. After time  $\tau$  we bring the qubit 2 energy quickly up through the filter and then adiabatically back down, which converts the filter photon back into a qubit excitation. Finally, we measure the qubit 2 state. Since no microwave excitation pulse is applied to qubit 2, it can only be excited by retrieving a photon from the filter. The resulting data from this measurement is outlined in Fig. 6. The data shows a clear exponential decay from the cavity that we can fit to extract a lifetime of  $2.65\mu\text{s}$  ( $Q = 1.16 \times 10^5$ ). This is consistent with directly measuring the low-power linewidth of an individual filter cavity.

## VII. CONTROLLED-Z GATE CALIBRATION

The controlled-Z (CZ) “AMP” gate sequence discussed in the main text is shown in detail in Fig. 7. The gate is designed to generate a state dependent interaction such that the qubit 1 excited state acquires a  $\pi$  phase if qubit

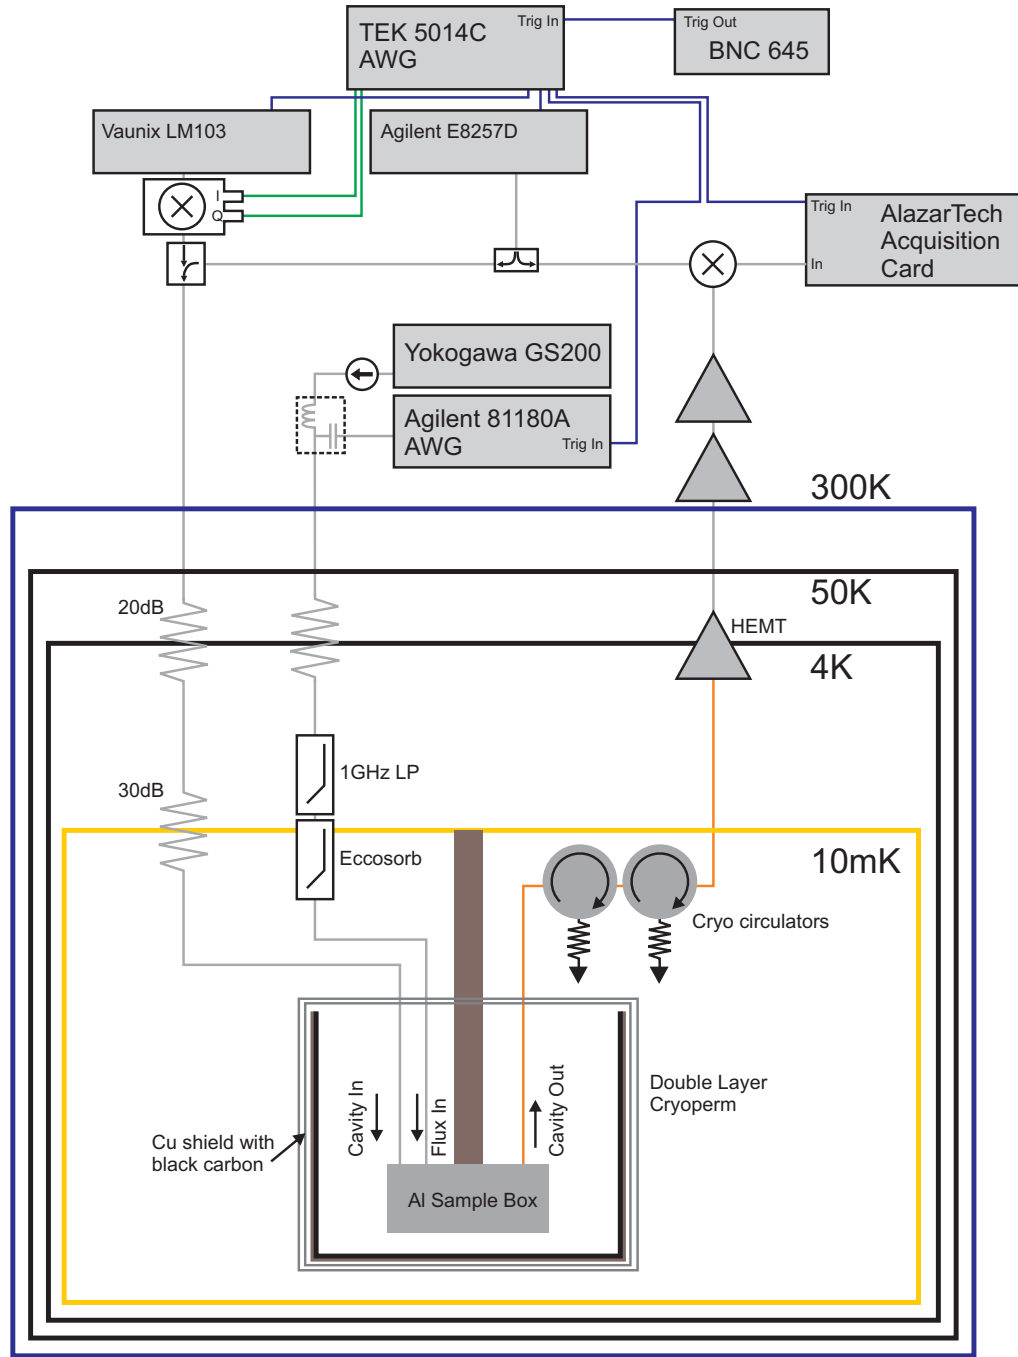

FIG. 4: Schematic of the instrumentation and cryogenic setup. Connecting lines are colour-coded: gray lines are coaxial cable (stainless steel inside the cryostat), orange lines are NbTi superconducting coaxial cable, green lines are analog control signals, and blue lines are digital control signals. The sample is mounted to the base stage of a dilution refrigerator with filtered microwave and DC connections to room temperature. For clarity, only qubit 1 connections are illustrated. Two microwave signals, the drive tone and the measurement tone, are sent down to the qubit and are attenuated at the 4K and 10mK stages for thermalization. Drive pulses are shaped using an IQ mixer, which is controlled by a Tektronix (TEK) 5014 arbitrary waveform generator (AWG). The measurement tone back from the qubit goes through a set of two cryo-circulators and is amplified at 4K. The signal is amplified again at room temperature and then mixed with a local oscillator (homodyne detection) and measured using a fast ADC. The DC qubit flux is provided by a stable DC current source which is filtered and passed through the DC port of a bias tee. Fast-flux pulses are provided by an Agilent 81180A 4.2GSa/s AWG which is connected to the RF port of the bias tee. Importantly, all flux signals are floating (see §V for more details). Each experimental cycle is instigated by a master trigger, which starts a sequence on the TEK AWG. All other instruments are controlled from the TEK AWG. All instruments are referenced to a common 10MHz atomic clock.

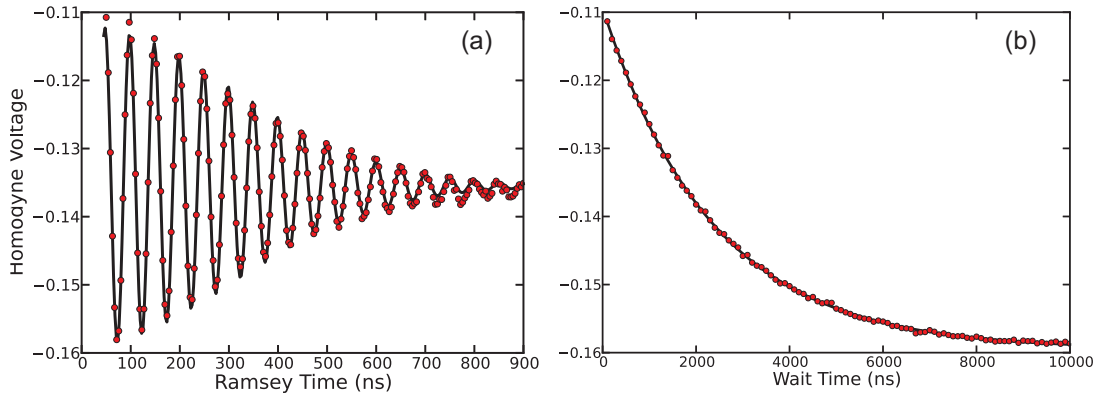

FIG. 5: Sample coherence and lifetime data for qubit 1. (a) Ramsey measurement without spin echo fit to Gaussian decay, and (b) lifetime measurement fit to exponential decay.

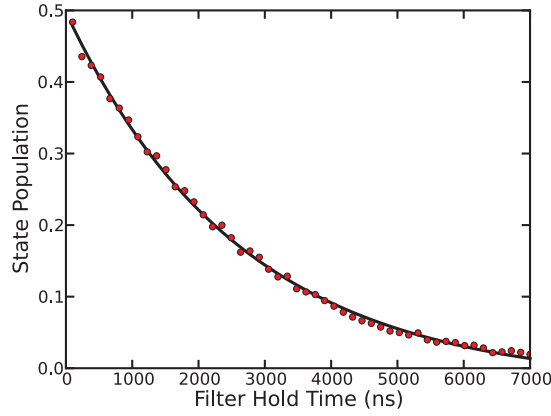

FIG. 6: Single-photon lifetime in the lowest filter mode. The data measures the qubit 2 state after retrieving a photon held in the filter for time  $\tau$ . The black solid line is an exponential fit.

2 is in the ground state. Because the qubit energies vary over a wide range there is also a large single-qubit phase (in the rotating frame at the qubit starting energies). The flux pulse is designed so that the single-qubit phase for the excited state of qubit 1 is  $\pi$  (modulo  $2\pi$ ). The single-qubit phase of qubit 2 is not calibrated and is given by  $\phi$ . Resonant microwave pulses are applied before and after the flux pulse to provide single qubit rotations around the X or Y axes of the Bloch sphere (depending on the IQ amplitude of the drive field).

To create the Bell state  $(|gg\rangle + e^{i\phi}|ee\rangle)/\sqrt{2}$  discussed in the main text we first apply  $\frac{\pi}{2}$  pulses to both qubits to prepare the state  $(|gg\rangle + |eg\rangle + |ge\rangle + |ee\rangle)/2$ . After the AMP gate, the state is ideally  $(|gg\rangle - |eg\rangle + e^{i\phi}|ge\rangle + e^{i\phi}|ee\rangle)/2$ , which can be rewritten in the form  $(|g\rangle - |e\rangle)/2 \otimes |g\rangle + e^{i\phi}(|g\rangle + |e\rangle)/2 \otimes |e\rangle$ . A second  $\frac{\pi}{2}$  pulse on qubit 1 rotates this to the desired Bell state  $(|gg\rangle + e^{i\phi}|ee\rangle)/\sqrt{2}$ . To create this Bell state we must calibrate two phases and the various single qubit rotations.

### A. Microwave Pulse Calibration

We perform arbitrary rotations around the X and Y axes of the Bloch sphere using resonant microwave pulses of arbitrary amplitude and phase. Pulse shaping and phase control is achieved by applying a voltage signal from an arbitrary waveform generator (Tektronix 5014C) to the two channels of an IQ mixer (Marki IQ0618LXP). We use Gaussian pulses that go to zero at  $\pm 2\sigma$ ; the AWG voltage applied to the mixer is,

$$V(t) = \begin{cases} V_0 \frac{e^{-(t-t_0)^2/2\sigma^2} - e^{-2}}{1 - e^{-2}} & , |t - t_0| \leq 2\sigma \\ 0 & , |t - t_0| > 2\sigma \end{cases} \quad (21)$$

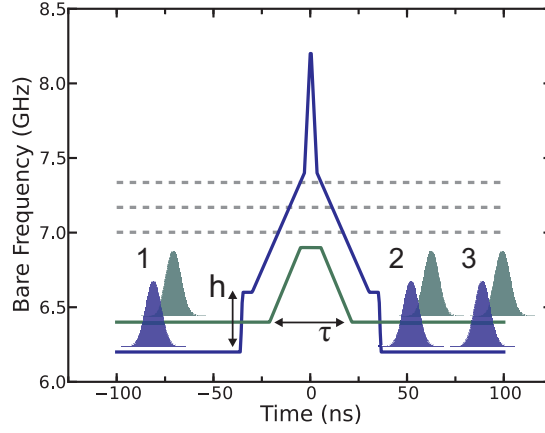

FIG. 7: AMP Gate sequence illustrating the flux pulses (solid lines) and microwave pulses (solid Gaussians). Qubit 1 is shown in blue and qubit 2 in green. Microwave pulses are separated for clarity, but are overlapped in the experiment. The flux pulse timing is accurate, but the microwave pulse locations are exaggerated for clarity. In the experiment pulse 1 is at -47.5ns, pulse 2 at 47.5ns, and pulse 3 at 72.5ns. The microwave pulses at locations 1 and 2 are the  $\frac{\pi}{2}$  pulses required to create a Bell state. The microwave pulses at location 3 are for state tomography. The sharp peak in the qubit 1 flux pulse is not material to the gate performance and is omitted in the flux diagram in Fig. 4 of the main text for clarity.

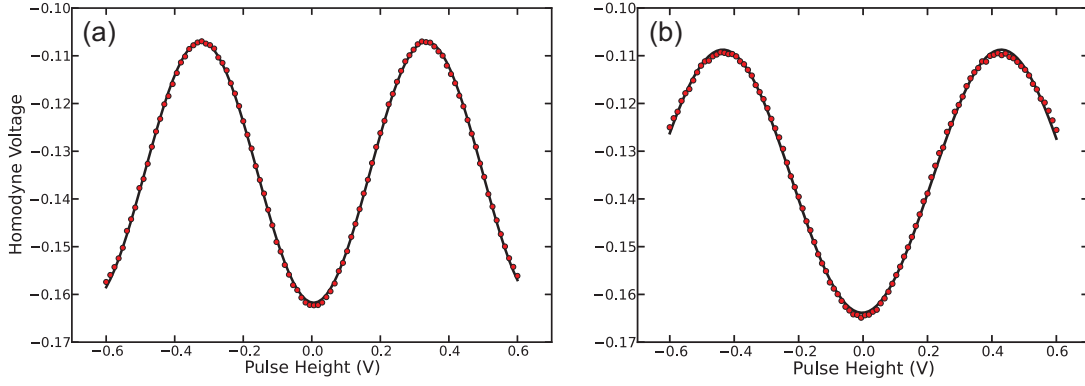

FIG. 8: Sample microwave pulse calibration data for qubit 1 at location 3 in Fig. 7 for the I (a) and Q (b) quadratures. We measure the homodyne voltage versus the microwave pulse height (in units of the analog voltage applied to the mixer I/Q port). The data is fit to a sinusoid (solid black line).

where  $V_0$  is adjusted to set the rotation angle. For all the pulses in our experiment we set  $\sigma = 5$ ns, so our total single-qubit gate time is 20ns. For this value of  $\sigma$  we find negligible difference between Gaussian and DRAG[4] pulses.

To calibrate the pulse height  $V_0$  we perform a Rabi oscillation at the given pulse location in the full gate sequence (setting all other microwave pulses to zero). We fit this oscillation to a sinusoid and identify the value of  $V_0$  associated with the sinusoid acquiring  $\pi$  phase as the  $\pi$ -pulse and similarly for the  $\frac{\pi}{2}$  pulse. Sample data is shown in Fig. 8.

## B. Flux Pulse Calibration

There are two free parameters for the flux pulse component of the gate, the height of the qubit 1 flux pedestal  $h$ , and the time of the qubit 2 flux pulse  $\tau$  (see Fig. 7). The other parameters of the flux pulse are fixed, but have been empirically optimized to maximize fidelity. For example, the total time of the qubit 1 flux pulse is set to be as short as possible to minimize decoherence while remaining adiabatic. The height of the qubit 2 pulse is set to maximize the c-phase rate for the transmon, which occurs when the qubit is brought just below the filter [5].

To calibrate  $h$  we measure the state of qubit 1 (applying  $\frac{\pi}{2}$  pulses to qubit 1 before and after the flux pulse) as a function of  $h$  with qubit 2 in  $|e\rangle$ . This is similar to the gate sequence, except that the  $\frac{\pi}{2}$  pulse for qubit 2 is instead a

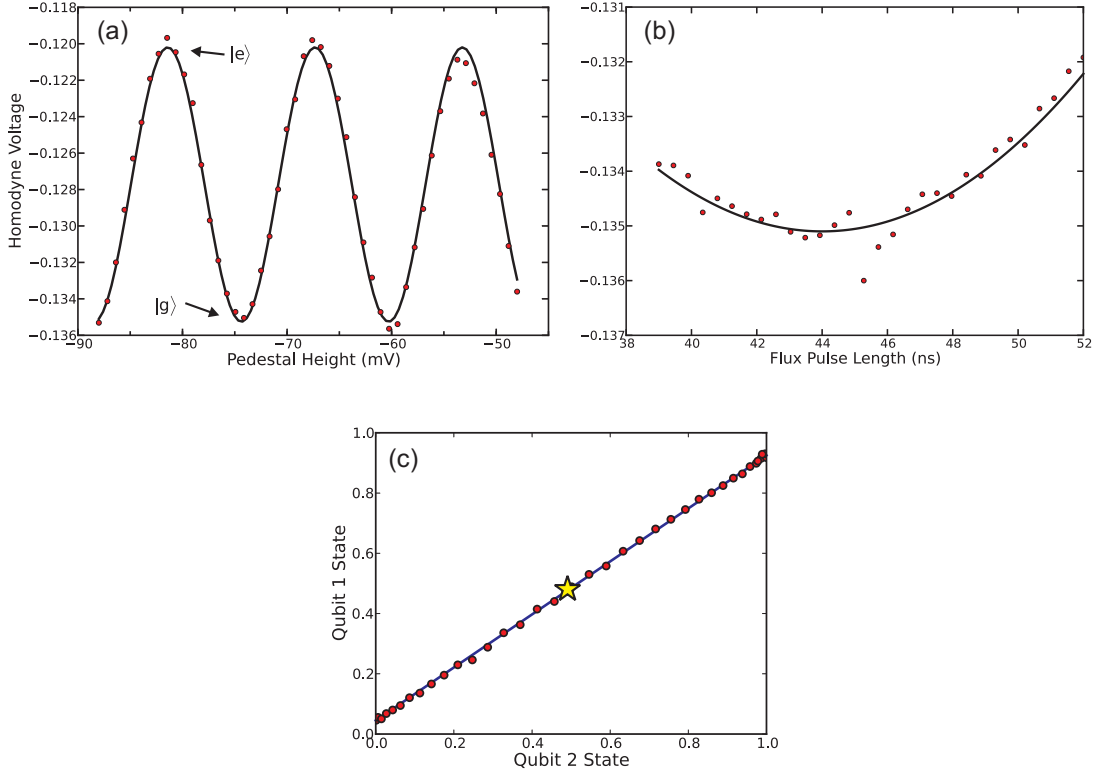

FIG. 9: (a) Calibrating the pedestal height  $h$ . (b) Calibrating the qubit 2 flux pulse length  $\tau$ . (c) To confirm the flux pulse calibration we perform a Ramsey measurement on qubit 1 and a Rabi oscillation on qubit 2. With qubit 2 in state  $|g\rangle$  we recover the state  $|gg\rangle$  and with qubit 2 in state  $|e\rangle$  we get  $|ee\rangle$  as expected for a properly calibrated sequence. The state highlighted by  $*$  is a candidate Bell state, but to confirm we need full state tomography (§VIII).

$\pi$  pulse. Data for this calibration are shown in Fig. 9. We select the value of  $h$  corresponding to qubit 1 in  $|e\rangle$  (i.e., the total two-qubit state is  $|ee\rangle$ ). Next, we vary  $\tau$  with qubit 2 in  $|g\rangle$ . We select the value of  $\tau$  corresponding to qubit 1 in  $|g\rangle$ . For the selected height of the qubit 2 pulse, the qubit 1 state is relatively insensitive to  $\tau$  as shown in Fig. 9. Fortunately, these calibrations are relatively orthogonal. To confirm the calibration we measure qubit 1 (applying  $\frac{\pi}{2}$  pulses on qubit 1 before and after the flux pulse) as a function of the qubit 2 state (by varying the qubit 2 pulse height before the flux sequence). This data is illustrated in Fig. 9.

### VIII. READOUT AND STATE TOMOGRAPHY

To measure the two-qubit state (after a particular gate sequence) we record the homodyne voltage (averaged over 600ns) for each qubit (see Fig. 4) from every run. For example, run  $i$  of the experiment would result in a voltage pair  $(V_{1,i}, V_{2,i})$ . These voltages are random numbers generated from a specific distribution corresponding to both quantum (i.e. projection) noise and experimental noise (mostly thermal noise from the HEMT amplifier). To measure the population in the four two-qubit basis states —  $|gg\rangle, |eg\rangle, |ge\rangle, |ee\rangle$  — we construct the histograms for these states by applying  $\pi$  pulses to the qubits at location 3 in Fig. 7 (all other pulses are set to zero). These histograms approximate the probability distribution for measuring a given voltage pair when the system is in a given basis state, which we represent by the function  $F_i(V_1, V_2)$  where  $i = \{|gg\rangle, |eg\rangle, |ge\rangle, |ee\rangle\}$ . Sample histograms are illustrated in Fig. 10. We select the frequency, power, and integration window of the homodyne measurement to empirically optimize the histograms in Fig. 10. For an unknown density matrix  $\rho$  we construct the histogram for  $\rho$  from  $N$  measurements,  $G_\rho(V_1, V_2)$ , and project onto the histograms for the basis states. To project we construct the matrix

$$\mathbf{A}_{ij} = \int \int dV_1 dV_2 F_i(V_1, V_2) F_j(V_1, V_2), \quad (22)$$

and vector

$$\mathbf{B}_i = \int \int dV_1 dV_2 F_i(V_1, V_2) G_\rho(V_1, V_2), \quad (23)$$

so that the vector

$$\mathbf{P} = \mathbf{A}^{-1} \cdot \mathbf{B} \quad (24)$$

gives the diagonal elements of  $\rho$ , i.e., the probabilities to be in all the basis states. For a finite number of measurements (of  $\rho$  and the basis states) Eqn. 24 gives an estimate of the true probabilities. We model the measurement using Monte Carlo to determine the statistical errors in this process (see §VIII A).

We perform state tomography using the standard method (see, e.g., Ref. [6]) by calculating the linear estimator,

$$\rho_{est} = \sum_{i,j} \frac{\text{Trace}[(\sigma_i \otimes \sigma_j) \rho] (\sigma_i \otimes \sigma_j)}{4}. \quad (25)$$

To calculate the term  $\text{Trace}[(\sigma_i \otimes \sigma_j) \rho]$  in Eqn. 25 we apply a unitary operator  $U$  to  $\rho$  (i.e.,  $\rho_2 = U \rho U^\dagger$ ) and then measure the diagonal elements of  $\rho_2$  using the procedure defined by Eqn. 24. To use a single qubit as an example, we can measure  $\text{Trace}[\sigma_Z \rho]$  directly,

$$\text{Trace}[\sigma_Z \rho] = P_e - P_g \quad (26)$$

where  $P_e - P_g$  is given by Eqn. 24. Then, to measure the other two trace terms, we apply a  $\frac{\pi}{2}$  rotation around the  $X$  and  $Y$  axes,

$$\text{Trace}[\sigma_X \rho] = \text{Trace}[\sigma_Z (R_Y(-\pi/2) \rho R_Y(\pi/2))], \quad (27)$$

$$\text{Trace}[\sigma_Y \rho] = \text{Trace}[\sigma_Z (R_X(-\pi/2) \rho R_X(\pi/2))]. \quad (28)$$

For two-qubits, there are nine required measurements corresponding to the following unitary operators on  $\rho$ ,  $(I, R_Y(\pi/2), R_X(\pi/2)) \otimes (I, R_Y(\pi/2), R_X(\pi/2))$ .

The linear estimator (Eqn. 25) can return unphysical results because it projects onto the space of all Hermitian matrices with  $\text{Trace} = 1$  whereas the density matrix must also be positive semi-definite. Following the maximum-likelihood protocol outlined in Ref. [6], we estimate the most likely physical density matrix by minimizing the function,

$$F[\rho_{est}] = \sum_{i=1, j=1}^{N,4} \left( \langle j | U_i^\dagger \rho_{est} U_i | j \rangle - P_{i,j} \right)^2 \quad (29)$$

where  $U_i$  are the set of  $N$  applied tomography pulses,  $|j\rangle$  is the  $j^{th}$  basis state,  $P_{i,j}$  is the measured probability, and  $\rho_{est}$  is a physical density matrix. The starting guess for the minimization is the density matrix estimated from Eqn. 25 with all negative eigenvalues set to zero. When using Eqn. 29 to estimate  $\rho$   $N \geq 9$ , so we also measure the negative pulse set [7]  $(I, R_Y(-\pi/2), R_X(-\pi/2)) \otimes (I, R_Y(-\pi/2), R_X(-\pi/2))$  for a total of 17 tomography measurements.

## A. Monte Carlo Simulation

To estimate the statistical and systematic errors in our state tomography, we generate test data from a known density matrix and analyze the data using the procedure described above. To generate the test data we start from density matrix  $\rho$  and apply the set of 17 single qubit rotations corresponding to the positive and negative tomography pulses to create 17 density matrices  $\rho_i = U_i \rho U_i^\dagger$ ; we also include density matrices for the four basis states (i.e.,  $\rho_j = |j\rangle\langle j|$ ). From these 21 density matrices we simulate  $N$  measurements. First, we randomly select the state of the qubit using the probabilities from the diagonal elements of  $\rho_i$  — this simulates the quantum projection noise. Then a voltage pair is randomly generated from the probability distribution corresponding to the selected basis state — this simulates the measurement noise. The probability distributions are designed to match the data in Fig. 10.

To estimate statistical errors we start with the density matrix  $\rho_{test} = 0.92|\Psi_{Bell}\rangle\langle\Psi_{Bell}| + 0.0064|gg\rangle\langle gg| + 0.0368|ge\rangle\langle ge| + 0.0368|eg\rangle\langle eg|$  which represents a Bell state with T1 decay. This state has a fidelity of  $F = 0.925$

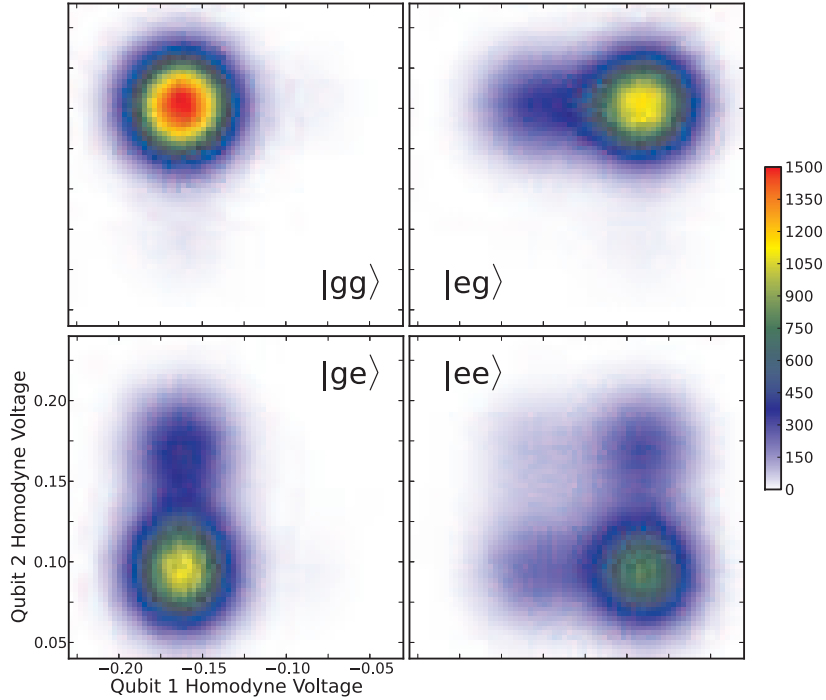

FIG. 10: 2D Histograms ( $70 \times 70$  bins) of the detector homodyne voltages for  $5 \times 10^5$  experiment runs with the qubits in the four basis states. The width of the distributions is due to noise in the measurement which is dominated by the thermal noise from the HEMT amplifier. There is also decay during the measurement since the measurement time of 600ns is on the order of  $T_1$ .

(with  $|\Psi_{\text{Bell}}\rangle$ ) and a concurrence of  $C=0.85$ . Similar to the experimental procedure, we take  $5 \times 10^5$  data points and then create histograms using  $25 \times 25$  bins and reconstruct the density matrix  $\rho_2$ . We then compute the concurrence and fidelity of  $\rho_2$  and repeat the procedure 50 times to build up statistics. There is no bias of the fidelity and concurrence and the standard deviation of each is 0.5% and 1.0%, respectively.

To estimate systematic errors we use  $\rho_{\text{test}}$  and incorporate random pulse rotation errors on the tomography pulses and on the pulses used to generate the basis states. For each run we select a random rotation error (for each pulse) from a uniform distribution bounded by a maximum rotation error. We then repeat 50 times to build up statistics on C, F, and the chi-square ( $\chi^2$ ) of the maximum likelihood estimator. For a rotation error bounded by  $\pm 7.5\%$  we find that the mean  $\chi^2$  of the simulation is similar to the  $\chi^2$  for the experimental state tomography data. The standard deviation of fidelity is 0.6% and concurrence is 1.3%. The mean fidelity is biased up by 0.3% and the concurrence by 0.8%.

## B. Process Tomography

To fully characterize the controlled-Z gate we perform process tomography. The procedure we follow is outlined in [8, 9]. We input a series of 16 states into the controlled-Z gate by performing different pulses at position 1 in Fig. 7 and measuring the resulting density matrix using state tomography. For the process tomography measurement we move the state tomography pulses from position 3 to position 2 in Fig. 7.

The process tomography procedure determines the matrix  $\chi$  which maps an input density matrix to an output density matrix as

$$\rho_f = \sum_{i,j} \chi_{i,j} \hat{E}_i \rho_i \hat{E}_j^\dagger \quad (30)$$

where  $\hat{E} = \{I, \sigma_X, -i\sigma_Y, \sigma_Z\} \otimes \{I, \sigma_X, -i\sigma_Y, \sigma_Z\}$  are the basis operators. The  $\chi$  matrix for our experiment is illustrated in Fig. 11.

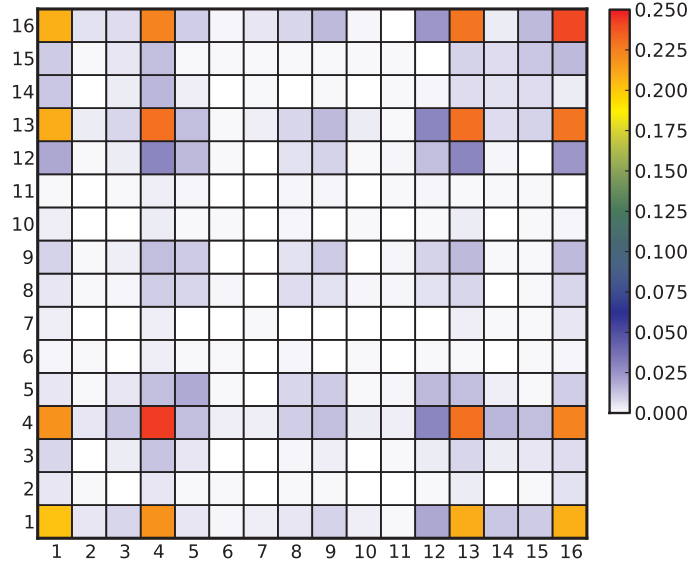

FIG. 11: Absolute value of the  $\chi$  matrix from process tomography. For the ideal CZ gate all the largest elements would be 0.25 and all other entries are zero.

To compare to the ideal case we use process fidelity,  $F_p = \text{Tr}(\chi_1 \chi_2)$  and the average gate fidelity  $\bar{F} = (dF_p + 1)/(d + 1)$  where  $d$  is the dimension of two-qubit space ( $d = 4$ ) [9]. From our process tomography  $F_p = 0.89$  and  $\bar{F} = 0.91$ .

### IX. MASTER EQUATION SIMULATION

To understand how decoherence limits our gate performance, we model the procedure of creating a Bell state by solving the master equation outlined in [10],

$$\dot{\rho}(t) = -\frac{i}{\hbar}[\hat{H}(t), \rho] + \mathcal{L}[\rho] \quad (31)$$

where  $\hat{H}(t)$  is the Hamiltonian for the qubit-filter system given in the main text with time-dependent qubit energies as illustrated in Fig. 7. The  $\frac{\pi}{2}$  pulses before and after the flux pulse are put into the simulation as discrete unitary operators. The second term in Eqn. 31 is the Lindblad operator that describe dephasing and decay,

$$\mathcal{L}[\rho] = \sum_i \mathcal{L}_i \rho \mathcal{L}_i^\dagger - \frac{1}{2} \left\{ \mathcal{L}_i^\dagger \mathcal{L}_i, \rho \right\} \quad (32)$$

where  $i$  is a sum over operators. The operator for the decay of qubit  $j$  is  $\mathcal{L}_{T_1,j} = \frac{\sigma_j^-}{\sqrt{T_1}}$  and for dephasing is  $\mathcal{L}_{T_2,j} = \frac{\sigma_j^z + 1}{2} \sqrt{\frac{2}{T_2}}$ .

If we simulate the Bell state procedure with only decay ( $2\mu\text{s}$  for the qubit,  $2.5\mu\text{s}$  for the filter), but no dephasing, we get a fidelity of  $F = 0.956$ . Simulating dephasing is less straightforward. Because we observe Gaussian decay of single qubit Ramsey fringes (see § IV), characterized by  $\sigma_{\text{decay}}$ , the dephasing time is not described by a single  $T_2$ . Instead, we set  $1/T_2 = 0$  in the master equation and simulate dephasing by adding a random frequency offset to each qubit where the frequency offset is selected from a normal distribution with  $\sigma_\omega = \sigma_{\text{decay}}^{-1}$ . Adding Ramsey fringes together with this type of frequency offset reproduces the observed Gaussian decay. We run the master equation simulation 20 times with these random offsets and average the density matrices. The resulting fidelity is 0.94. The effect of dephasing is minimized for two reasons. First, the time of the gate is short compared to  $\sigma_{\text{decay}}$ , and second,

when the excitation is in the filter it is unaffected by offsets to the qubit energy.

- 
- [1] D. Sank, R. Barends, R. C. Bialczak, Y. Chen, J. Kelly, M. Lenander, E. Lucero, M. Mariantoni, A. Megrant, M. Neeley, et al., Phys. Rev. Lett. **109**, 067001 (2012).
  - [2] J. Koch, T. M. Yu, J. Gambetta, A. A. Houck, D. I. Schuster, J. Majer, A. Blais, M. H. Devoret, S. M. Girvin, and R. J. Schoelkopf, Phys. Rev. A **76**, 042319 (2007).
  - [3] B. Johnson, Ph.D. thesis, Yale University (2010).
  - [4] J. M. Chow, L. DiCarlo, J. M. Gambetta, F. Motzoi, L. Frunzio, S. M. Girvin, and R. J. Schoelkopf, Phys. Rev. A **82**, 040305(R) (2010).
  - [5] L. Bishop, *Multipole theory paper*, To appear (2014).
  - [6] D. F. James, P. G. Kwiat, W. J. Munro, and A. G. White, Phys. Rev. A **64**, 052312 (2001).
  - [7] J. M. Chow, L. DiCarlo, J. M. Gambetta, A. Nunnenkamp, L. S. Bishop, L. Frunzio, M. H. Devoret, S. M. Girvin, and R. J. Schoelkopf, Phys. Rev. A **81**, 062325 (2010).
  - [8] M. A. Nielsen and I. L. Chuang, *Quantum Computation and Quantum Information* (Cambridge, 2000).
  - [9] J. L. O'Brien, G. J. Pryde, A. Gilchrist, D. F. V. James, N. K. Langford, T. C. Ralph, and A. G. White, Phys. Rev. Lett. **93**, 080502 (2004).
  - [10] T. Yamamoto, M. Neeley, E. Lucero, R. C. Bialczak, J. Kelly, M. Lenander, M. Mariantoni, A. D. OConnell, D. Sank, H. Wang, et al., Phys. Rev. B **82**, 184515 (2010).
